# Supplementary material for: Single-Bubble Dynamics in Nanopores: Transition Between Homogeneous and Heterogeneous Nucleation
Source: arXiv:2007.13063 ancillary file (2020-11-19)
Supplement: Supplementary file 1 [file Supplemental_information.pdf]

## Supplementary Material for

# "Single-Bubble Dynamics in Nanopores: Transition Between Homogeneous and Heterogeneous Nucleation"

Soumyadeep Paul[1], Wei-Lun Hsu,[1] Mirco Magnini,[2] Lachlan R Mason,[3] Ya-Lun Ho,[1] Omar K Matar,[4] and Hirofumi Daiguji[1]

[1]Department of Mechanical Engineering, The University of Tokyo, 7-3-1, Hongo, Bunkyo-ku, Tokyo 113-8656, Japan

[2]Department of Mechanical Engineering, University of Nottingham, Nottingham, NG7 2RD, United Kingdom

[3]Data-Centric Engineering Programme, The Alan Turing Institute, London, NW1 2DB, United Kingdom

[4]Department of Chemical Engineering, Imperial College London, London, SW7 2AZ, United Kingdom

## 1. SEM images of nanopores

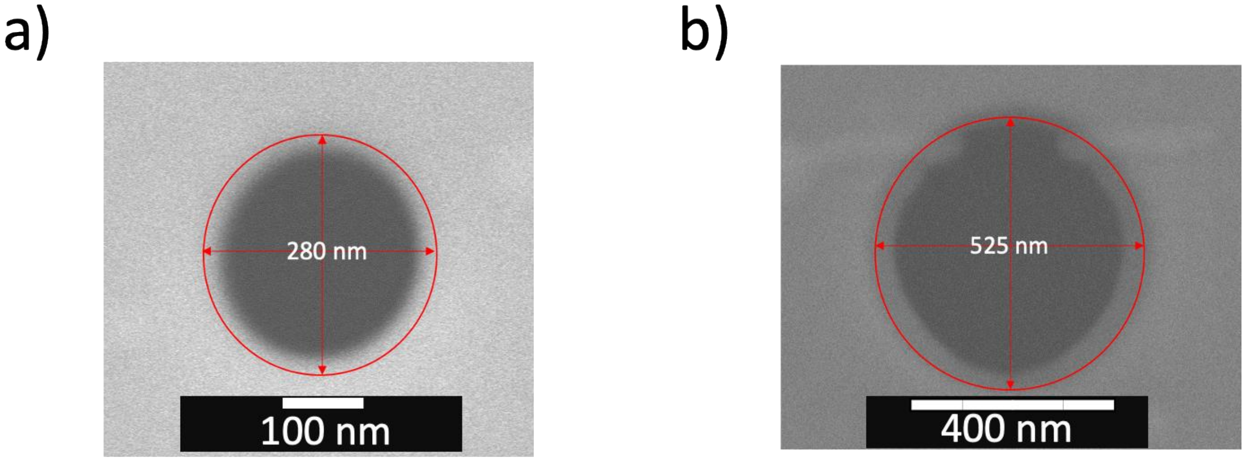


FIG. S1.1. SEM images of (a) a 280-nm-diameter pore and (b) a 525-nm-diameter pore.

These images were taken post-FIB fabrication and prior to piranha cleaning.

## 2. Nanopore Joule heating

According to Joule's law, the heat dissipation by Joule heating across a resistor is proportional to the product of the current flowing and the associated voltage drop.

$$\mathrm{JH} = V \times I \tag{S2.1}$$

The same concept can be applied to ionic currents in electrolytes. A small two-dimensional (2D) section (*dx* × *dy*) of electrolyte is shown in Fig. S2.1. Using Eq. (15), the total Joule heat JH dissipated in the section, *dxdy*, can be mathematically expressed as

$$\mathrm{JH} = V_x \times I_x + V_y \times I_y = E_x dx \times J_x dy + E_y dy \times J_y dx, \tag{S2.2}$$

$$H = \frac{\mathrm{JH}}{dxdy} = E_x \times J_x + E_y \times J_y = \sigma |\mathbf{E}|^2. \tag{S2.3}$$

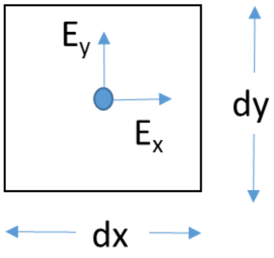


FIG. S2.1. A small 2D section of electrolyte.

The Joule heat density derived in Eq. (S2.3) serves as an energy-source term in the energy-conservation equation of the electrolyte.

$$\rho c_p \frac{\partial T}{\partial t} = \frac{1}{y}\frac{\partial}{\partial y}\left(\kappa y \frac{\partial T}{\partial y}\right) + \frac{\partial}{\partial z}\left(\kappa \frac{\partial T}{\partial z}\right) + \boldsymbol{J} \cdot \boldsymbol{E} \tag{S2.4}$$

The thermophysical properties of water, such as its specific heat capacity $c_\mathrm{p}$, density $\rho$, thermal conductivity $\kappa$, and dielectric constant $\epsilon$, were modeled as a function of liquid temperature [1–3] (Fig. S2.2).

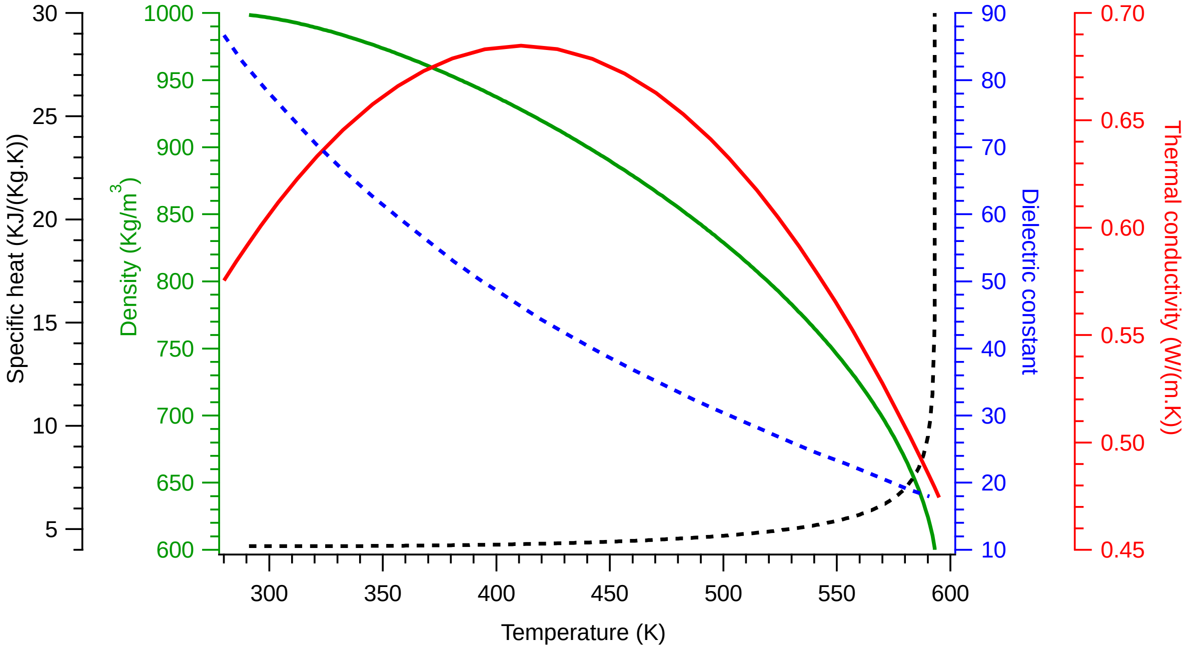


FIG. S2.2. Temperature dependence of water properties in the stable and metastable liquid phases.

The left-hand side term in Eq. (S2.4) measures the transient increase of the electrolyte's internal energy, and the first two terms on the right-hand side accounts for thermal diffusion in $y$ and $z$ directions respectively. The Joule heat-source term couples the energy equation with the electrokinetics of the nanopore. Joule heat generation in the bulk electrolyte is accompanied by heat dissipation through the silicon nitride membrane, which is in close proximity to the pore region. This can be solved by

$$\rho_{\mathrm{SiN}x} c_{\mathrm{SiN}x} \frac{\partial T}{\partial t} = k_{\mathrm{SiN}x} \left( \frac{1}{y} \frac{\partial}{\partial y} \left( y \frac{\partial T}{\partial y} \right) + \frac{\partial^2 T}{\partial z^2} \right). \quad \text{(S2.5)}$$

Here, $\rho_{\mathrm{SiN}x} = 3100$ Kg/m$^3$, $c_{\mathrm{SiN}x} = 700$ J/(Kg K), $k_{\mathrm{SiN}x} = 3.2$ W/(m K) are the density, specific heat, and thermal conductivity of silicon nitride adapted from Levine *et al.* [1]. In addition to the energy-transport equations, the nanopore electrokinetics need to be solved to obtain the variation of the ion flux and the electric-field distribution. Following the model presented in

Levine *et al.* [1], the ion flux is considered to be proportional to the electric field and can be expressed as

$$\boldsymbol{J} = \sigma \boldsymbol{E}. \tag{S2.6}$$

Here, $\sigma$ is the ionic conductivity of the electrolyte (3M NaCl), which was modeled by the empirical relationship [1]

$$\sigma = mT - b - \frac{(T-293.15)^{\alpha}}{\beta}. \tag{S2.7}$$

The values of $m = 0.391$ and $b = 96.9$ were obtained by Levine *et al.* [1] by fitting the experimentally obtained bulk electrical conductivity of 3M NaCl. The values of $\alpha = 2.7$ and $\beta = 5.6 \times 10^4$ were obtained in a previous study [1] by fitting the experimentally obtained nanopore conductance during Joule heating for a 107-nm-diameter pore. The first two terms in Eq. (S2.7) denote linear dependence of $\sigma$ upon $T$, as the mobility of the ions increases with temperature [4–6]. The last term on the right-hand side denotes a compensating effect that arises from ion-concentration reduction due to the density of water reducing with temperature [1,7]. In our Joule-heating experiments for the 525-nm- and 280-nm-diameter pores, we set $\alpha = 2.52$ and $\alpha = 2.3$ to fit the conductance of our experimental pores ($C = \frac{i}{V_{\text{app}}}$) for bias voltages without bubble generation [Figs. S2.3(b) and S2.3(c)].

To determine the nanopore electrokinetics, Eq. (S2.6) was solved, along with the ion-conservation equation, which can be written as

$$\nabla \cdot \boldsymbol{J} + \frac{\partial \rho_{\text{e}}}{\partial t} = 0, \tag{S2.8}$$

where the ionic charge density $\rho_{\text{e}}$ is related to the electric field according to the Poisson equation as

$$\rho_{\text{e}} = \nabla \cdot \epsilon \epsilon_0 \boldsymbol{E}, \tag{S2.9}$$

where $\epsilon_0$ is the permittivity of free space.

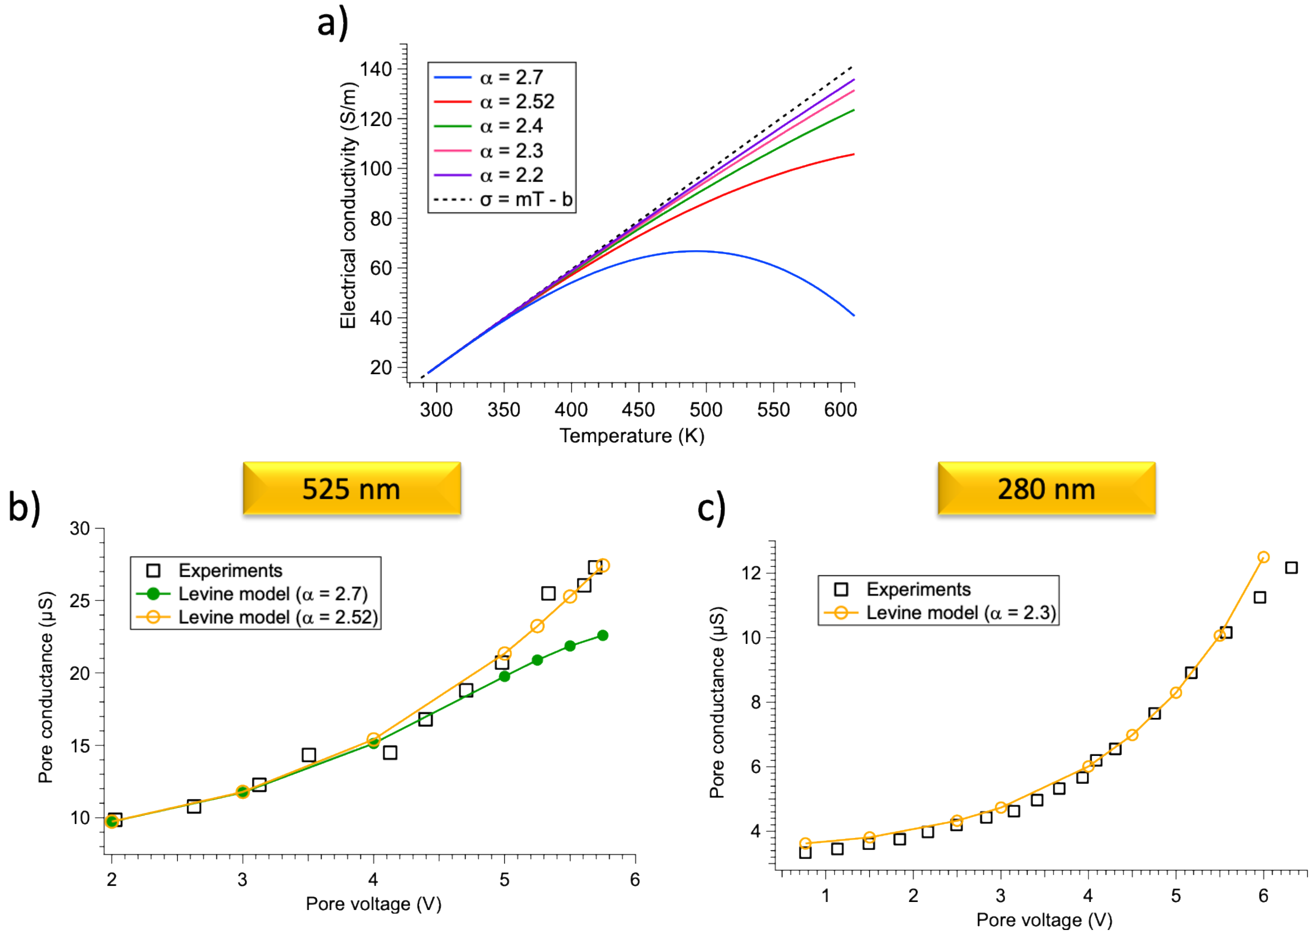


FIG. S2.3. (a) Temperature dependence of electrical conductivity of 3M NaCl solution, (b) effect of Joule heating on pore conductance for different pore voltages for the 525-nm-diameter pore, (c) effect of Joule heating on pore conductance for different pore voltages for the 280-nm-diameter pore. The conductance values for both experiments and simulations were measured 500 μs after the start of the voltage pulse.

Numerical simulations were used to solve the energy equations [Eqs. (S2.4) and (S2.5)] and the ion-transport equations [Eqs. (S2.6)–(S2.9)] on a 2D mesh using the finite-volume solver, ‘arb’ [8]. The fluidic connection through the nanopore is axisymmetric. We applied symmetric boundary conditions for the ion flux and the temperature gradient along the pore centerline [Fig. S2.4(a)]. On the silicon nitride walls and top face, a zero ion-flux boundary condition was

used. At the liquid–$Si_3N_4$ interface, the temperature and heat flux were continuous, i.e., $T_{\text{liquid side of interface}} = T_{\text{Si}_3\text{N}_4\text{ side of interface}}$. For the boundary edges of the nanopore system, ambient-temperature boundary conditions were used, i.e., $T = T_0$. Constant electric potential values were applied at the inlet and outlet faces [Fig. S2.4(a)], i.e., $V = -V_{\text{app}}/2$ and $V = V_{\text{app}}/2$ on the inlet and outlet faces, respectively. The nanopore area and a thin layer surrounding the $Si_3N_4$ membrane were discretized finely using a structured mesh, while the rest of the electrolyte area was discretized using an unstructured mesh. The whole $Si_3N_4$ surface was discretized using a structured mesh with a high mesh density along the electrolyte boundary. Inside the nanopore area, the mesh sizes were of the order of 1 nm. The mesh of the nanopore system is shown in Fig. S2.4(b).

Before simulating Joule heating in the nanopore, we first solved for the steady-state electric potential $V$ in the nanopore system by solving only the ion-transport equations, [Eqs. (S2.6)–(S2.9)]. For this step, the values of $\epsilon$ and $\sigma$ were constant and were calculated at ambient temperature, $T_0$. The solution of this simulation was used as the initial conditions for transient Joule heating. The time steps were designed to gradually increase from 10 fs as the simulation progressed according to

$$\Delta \mathrm{t} = 10^{-(7\exp(-0.01(n-1))+7)}, \tag{S2.10}$$

Here, *n* denotes the index of the time step. For Joule heating simulations intended for measuring nucleation temperature at the nucleation points only Eq. (S2.10) was used however, for the Joule heating simulations for measuring pore conductance at 500 µs as shown in Fig. S2.3(b,c) higher time step spacings were used for $n > 520$ according to

$$\Delta \mathrm{t} = 10^{-(6-0.00145*(n-520))} \tag{S2.11}$$

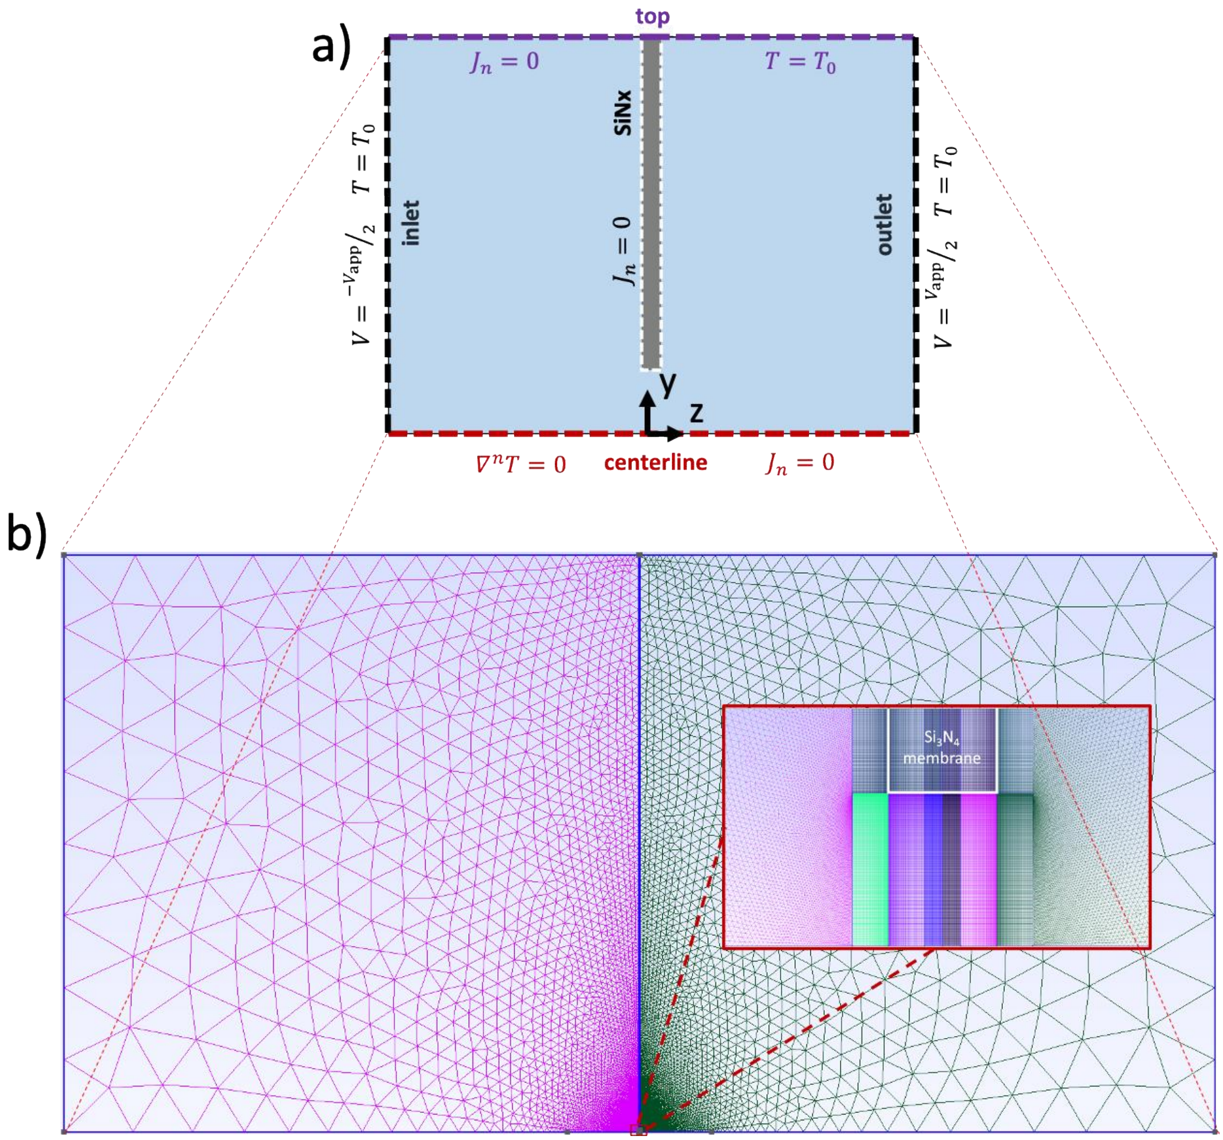


FIG. S2.4. (a) Schematic of the nanopore system showing the boundary conditions of temperature and ion flux that were applied to the nanopore simulation. $V_{\mathrm{app}}$ is the applied bias voltage, $T_0 = 300.15$ K and $T_0 = 296.55$ K are the ambient temperatures for the 525-nm and 280-nm pore experiments, and $J_{\mathrm{n}}$ is the face-normal ion flux. The simulation domain extended to 75 µm in the *y* and *z* directions. (b) Computational fluid dynamics mesh of the nanopore system for the 280-nm pore and the high mesh density inside the nanopore (inset). There are 314316 cells in the entire simulation domain.

# 3. Validation of nanopore current with simulations

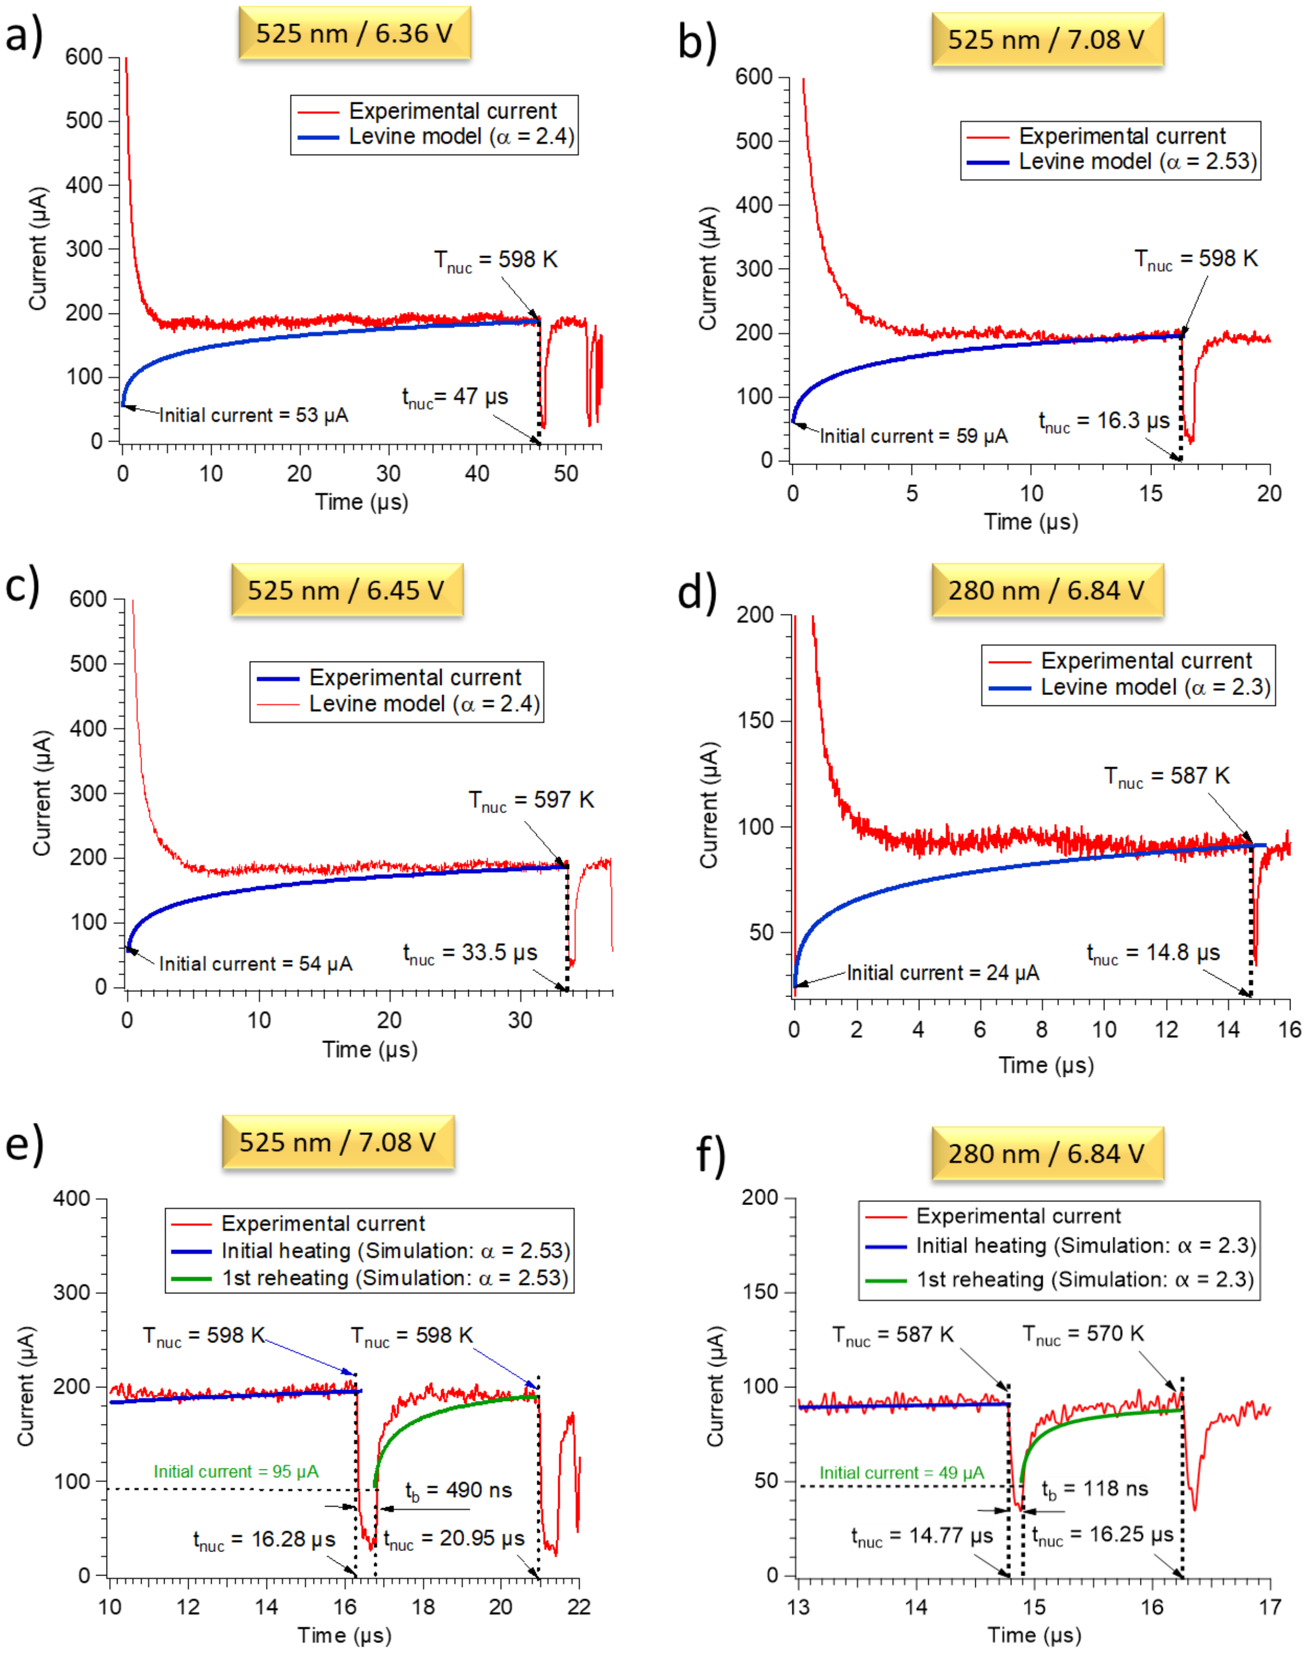

FIG. S3.1. Experimental (red) and simulation (blue) current traces during initial heating for bias voltages of (a) 6.36 V, (b) 7.08 V, and (c) 6.45 V across the 525-nm-diameter pore, and (d) 6.84 V across the 280-nm-diameter pore. The nanopore current was measured according to $i = \frac{V_\mathrm{s}}{R_\mathrm{s}}$, where $V_\mathrm{s}$ is the shunt voltage measured by the oscilloscope across the shunt resistance, $R_\mathrm{s}$. The bias voltage across the nanopore (or pore voltage), $V_\mathrm{app}$ was calculated according to $V_\mathrm{app} = V_{\mathrm{p}_\mathrm{avg}} - V_{\mathrm{s}_\mathrm{avg}}$, where $V_{\mathrm{p}_\mathrm{avg}}$ and $V_{\mathrm{s}_\mathrm{avg}}$ are the time-averaged pulse voltage and shunt voltage, respectively, starting from $t = t_0$ to $t = t_\mathrm{nuc}$. Here, $t_0$ is the time where the capacitance relaxation of the shunt voltage or current ends, which is 6 µs for the 525-nm results and 4 µs for the 280-nm results. This relaxation effect arises due to capacitive charging of the dielectric $Si_3N_4$ membrane and accumulation of depletion layers inside the Si frame supporting the membrane. Different parasitic contributions are involved in this capacitive charging [9], which makes modeling these effects in the presence of Joule heating more complicated. To avoid these complexities, we neglected the capacitive contributions in our simulations. As a result, the initial current was mismatched between the experiments and the simulations. Panels (e) and (f) represent matching of the experimental (red) and simulation (green) reheating current for 7.08 V across the 525-nm pore and 6.84 V across the 280-nm pore, respectively.

## 4. Transient traces for temperature development at pore center and pore walls

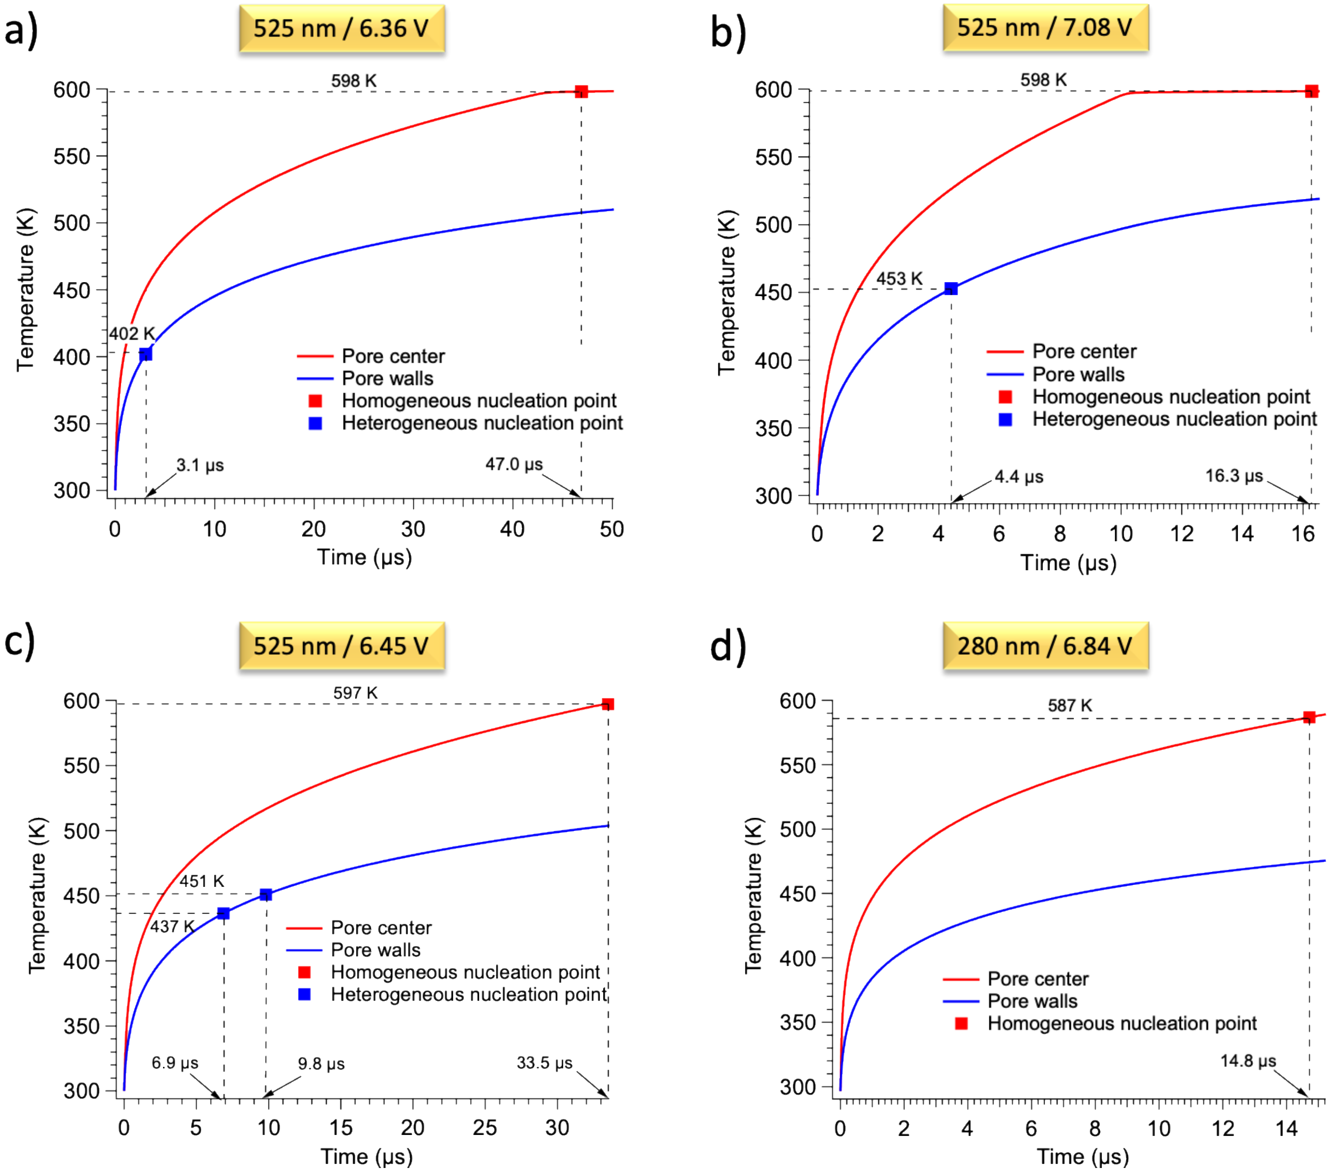


FIG. S4.1. Transient rise of the pore center and wall temperatures for (a) 6.36 V across the $D_p$ = 525 nm pore ($\alpha = 2.4$), (b) 7.08 V across the $D_p$ = 525 nm pore ($\alpha = 2.53$), (c) 6.45 V across the $D_p$ = 525 nm pore ($\alpha = 2.4$), and (d) 6.84 V across the $D_p$ = 280 nm pore ($\alpha = 2.3$). $\Delta T_p = T_c - T_w$ is higher for the 280-nm pore trace [panel (d)] than for the 525-nm pore traces [panels (a)–(c)] for a given time point.

# 5. Shape of a bubble on a cylindrical surface

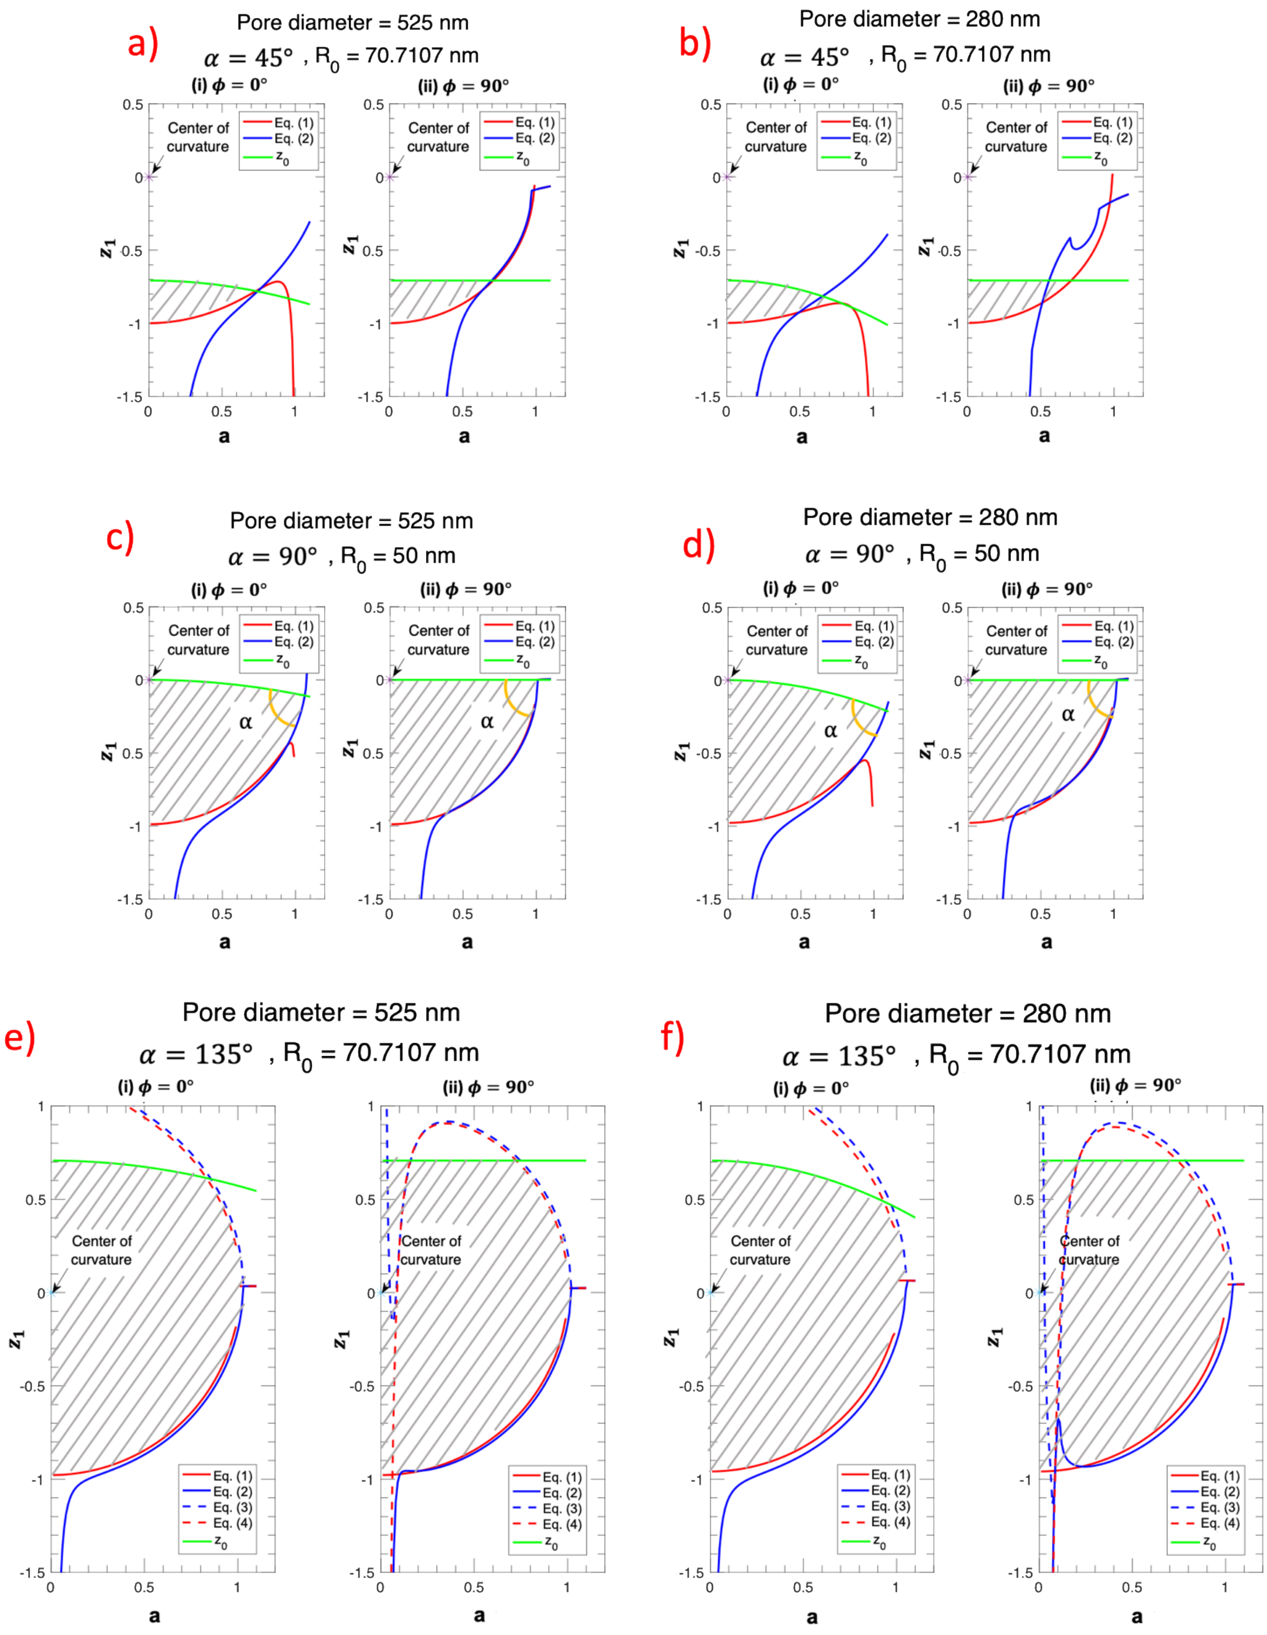

FIG. S5.1. Shape of a bubble on a curved surface for different pore diameters and radii. Sub-panels (i) and (ii) in each panel represent the cross-sectional image of the bubble along the $\phi = 0°$ and $\phi = 90°$ planes, respectively. Here, $\alpha = 180° - \theta$ is the bubble contact angle on the vapor side of the interface.

Soleimani *et al.* [10] derived the bubble shape on a cylindrical surface using domain perturbation theory. They started from a spherical cap of radius $R_0$ on a flat substrate and perturbed the flat substrate by a parameter $\varepsilon = -\frac{R_0}{R_\mathrm{p}}$, where $R_\mathrm{p}$ is the pore radius. For a flat surface, $R_\mathrm{p} \to \infty$, and so $\varepsilon \to 0$. As the substrate is perturbed, the bubble shape was solved subject to the constraints: i) constant volume, ii) uniform interface curvature, iii) $|\varepsilon| \ll 1$ and iv) validity of the Youg–Dupré condition at the contact line, $\gamma \cos \alpha = \gamma_\mathrm{sg} - \gamma_\mathrm{sl}$, where $\gamma$ is the surface tension at the liquid–gas interface, while $\gamma_\mathrm{sg}$ and $\gamma_\mathrm{sl}$ are the surface tensions at the solid–gas and solid–liquid interfaces, respectively. The perturbed shape of the bubble is captured by $z_1 = z_1(a, \phi)$ in the cylindrical co-ordinate system according to the four equations listed below. Here, $z_1$ is the normalized distance of a point on the bubble surface from the center of curvature along the bubble axis, and $a$ is the normalized radial distance from the bubble axis. The actual position of a point on the bubble surface is given by $Z_1 = R_0 z_1$ and $A = R_0 a$.

- For $\alpha < 90°$, the bubble surface is given by Eqs. (1) and (2). Two equations are needed as Eq. (1) becomes singular as $a \to 1$. Hence, for the range when Eq. (1) becomes singular, Eq. (2) is used to capture the bubble surface. To construct the bubble surface, we first check if Eq. (1) and $z_0$ have a root for a given value of $\phi$. If there is a root, then Eq. (1) is used to trace the bubble surface for the value of $\phi$. If Eq. (1) and $z_0$ have no common solution for a given value of $\phi$, then Eq. (2) is used to obtain the contact point with the pore surface. In this case, the bubble surface was mapped using Eq. (2) starting from the contact point until the point $(a, z_1)$ when $z_1$[Eq. (1)] = $z_1$[Eq. (2)] [Fig. S5.1(a)–(d)].

- For $\alpha > 90°$, the bubble surface can be divided into two cases:

    - Case 1: $z_1$[Eq. (4)] and $z_0$ do not have a root. The bubble surface is given by:
        - # In this part, the lower half of the bubble surface, i.e., the half closer to the walls, is mapped. In this range, $z_1(a) \leq z_1(a_\mathrm{max})$. Eq. (3) is used until $a = a_\mathrm{max}$.

- # In this part, the upper half of the bubble surface, i.e., the half closer to the pore center, is mapped. Eq. (1) is used for $a \geq a_{\max}$ for all values of $z_1$ where Eq. (1) is non-singular. For the range of $a$ in-between $[0, a_{\max}]$ where Eq. (1) becomes singular, Eq. (2) is used). At $a = a_{\max}$, $z_1$ [Eq. (2)] = $z_1$ Eq. (3)], as can be seen in Figs. S5.1(e) and S5.1(f).

- Case 2: $z_1$[Eq. (4)] and $z_0$ have a root. The bubble surface is given by:
  - # In this part, the lower half of the bubble surface, i.e., the half closer to the walls, is mapped. In this range, $z_1(a) \leq z_1(a_{\max})$. Eq. (4) is used for $a \leq a_{\max}$ for all values of $z_1$ where Eq. (4) is non-singular. For the range of $a$ where Eq. (4) becomes singular, Eq. (3) is used.
  - # In this part, the upper half of the bubble surface, i.e., the half closer to the pore center, is mapped. Eq. (1) is used for $a > a_{\max}$ for all values of $z_1$ where Eq. (1) is non-singular. For the range of $a$ in-between $[0, a_{\max}]$ where Eq. (1) becomes singular, Eq. (2) is used. At $a = a_{\max}$, $z_1$ [Eq. (2)] = $z_1$ [Eq. (3)], as can be seen in Figs. S5.1(e) and S5.1(f).

$$\text{Eq. (1): } z_1 = -\sqrt{1-a^2} + \varepsilon\left(C_0 + \frac{k}{2\sqrt{1-a^2}} + C_2\left(\frac{2}{a^2\sqrt{1-a^2}} - \frac{2}{a^2} - 1\right)\cos 2\phi\right) \tag{S5.1}$$

$$\text{Eq. (2): } z_1 = -\sqrt{1-a^2+\varepsilon\gamma_1(a,\phi)+\varepsilon^2\gamma_2(a,\phi)} + \varepsilon\gamma_3(a,\phi) \tag{S5.2}$$

$$\text{Eq. (3): } z_1 = \sqrt{1-a^2+\varepsilon\gamma_1(a,\phi)+\varepsilon^2\gamma_2(a,\phi)} + \varepsilon\gamma_3(a,\phi) \tag{S5.3}$$

$$\text{Eq. (4): } z_1 = \sqrt{1-a^2} + \varepsilon\left(C_0 - \frac{k}{2\sqrt{1-a^2}} - C_2\left(\frac{2}{a^2\sqrt{1-a^2}} + \frac{2}{a^2} + 1\right)\cos 2\phi\right) \tag{S5.4}$$

The equation of the perturbed pore surface is given by

$$z_0 = -\cos\alpha + \varepsilon\left[\frac{1}{4}a^2(1+\cos 2\phi)\right], \tag{S5.5}$$

and $a_{\max}$ is given by

$$a_{\max} = 1 + \varepsilon\frac{\gamma_1(1,\phi)}{2} + \varepsilon^2\left[\frac{\gamma_2(1,\phi)}{2} - \frac{\gamma_1(1,\phi)}{8}\right]^2, \tag{S5.6}$$

where the parameters $C_0$, $C_2$, $k$, $\gamma_1$, $\gamma_2$, and $\gamma_3$ are given by

$$C_0 = -\frac{1}{4}\sin^2\alpha - \frac{k}{2}\cos\alpha, \tag{S5.7}$$

$$C_2 = \frac{\sin^4\alpha}{24(1-\cos\alpha)-12\sin^2\alpha}, \tag{S5.8}$$

$$k = \frac{-3\sin^4\alpha}{4(2\cos\alpha-2+\sin^2\alpha\cos\alpha)}, \tag{S5.9}$$

$$\gamma_1(a,\phi) = -k - \frac{4C_2}{a^2}\cos 2\phi + \frac{1}{2}\left[\frac{1}{2} + \frac{2C_2}{a^2}\cos 2\phi\right]^2 \operatorname{sgn}(\varepsilon), \tag{S5.10}$$

$$\gamma_2(a,\phi) = \frac{1}{4}\left[\frac{k}{2} + \frac{2C_2}{a^2}\cos 2\phi\right]^2, \tag{S5.11}$$

$$\gamma_3(a,\phi) = C_0 - \left(\frac{2}{a^2} + 1\right) C_2 \cos 2\phi. \tag{S5.12}$$

## 6. Multi-pulse bubble generation results

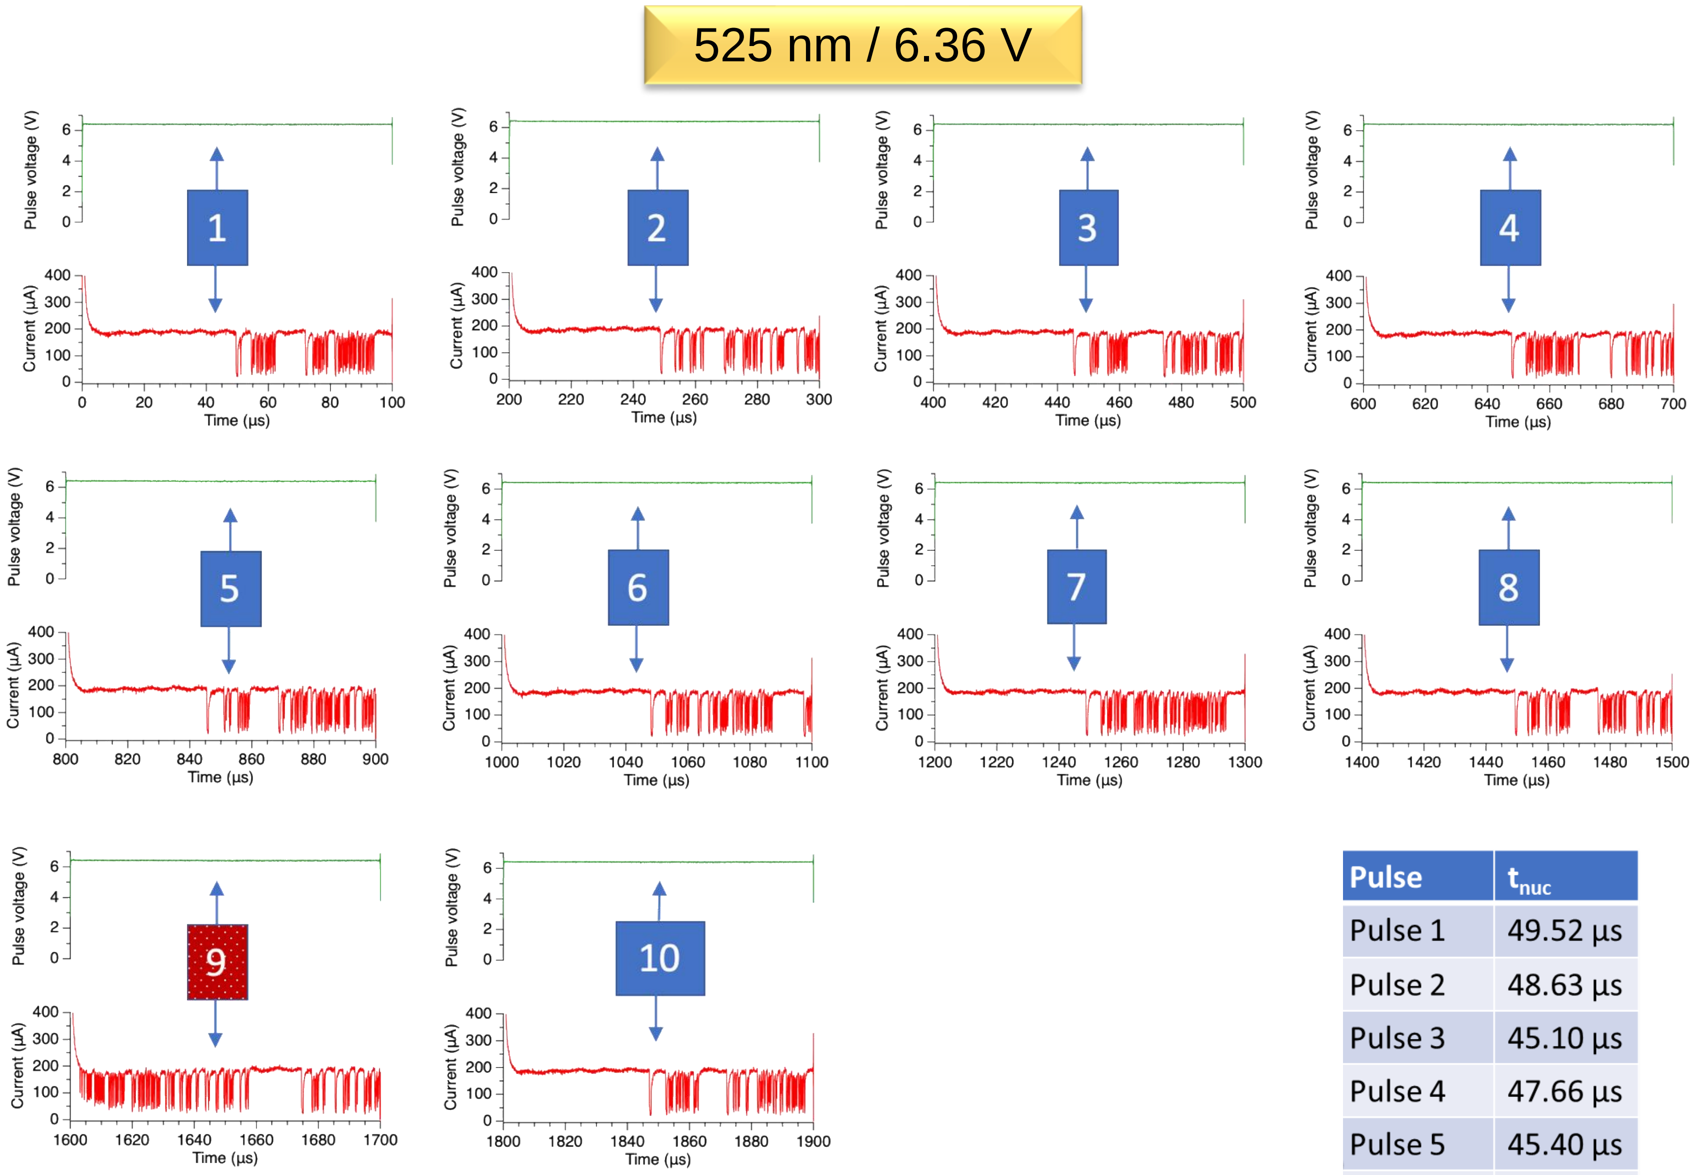


| Pulse | $t_{nuc}$ |
|---|---|
| Pulse 1 | 49.52 µs |
| Pulse 2 | 48.63 µs |
| Pulse 3 | 45.10 µs |
| Pulse 4 | 47.66 µs |
| Pulse 5 | 45.40 µs |
| Pulse 6 | 47.95 µs |
| Pulse 7 | 48.62 µs |
| Pulse 8 | 49.25 µs |
| Pulse 9 | 3.06 µs |
| Pulse 10 | 47.02 µs |

FIG. S6.1. Bubble-blockage signals for the 525-nm pore under a 6.36 V bias voltage and ten pulses. Early hetero nucleation is observed for only for one of these pulses, while for all the other pulses, there is a long waiting time, after which a homo bubble nucleates.

## 525 nm / 6.45 V

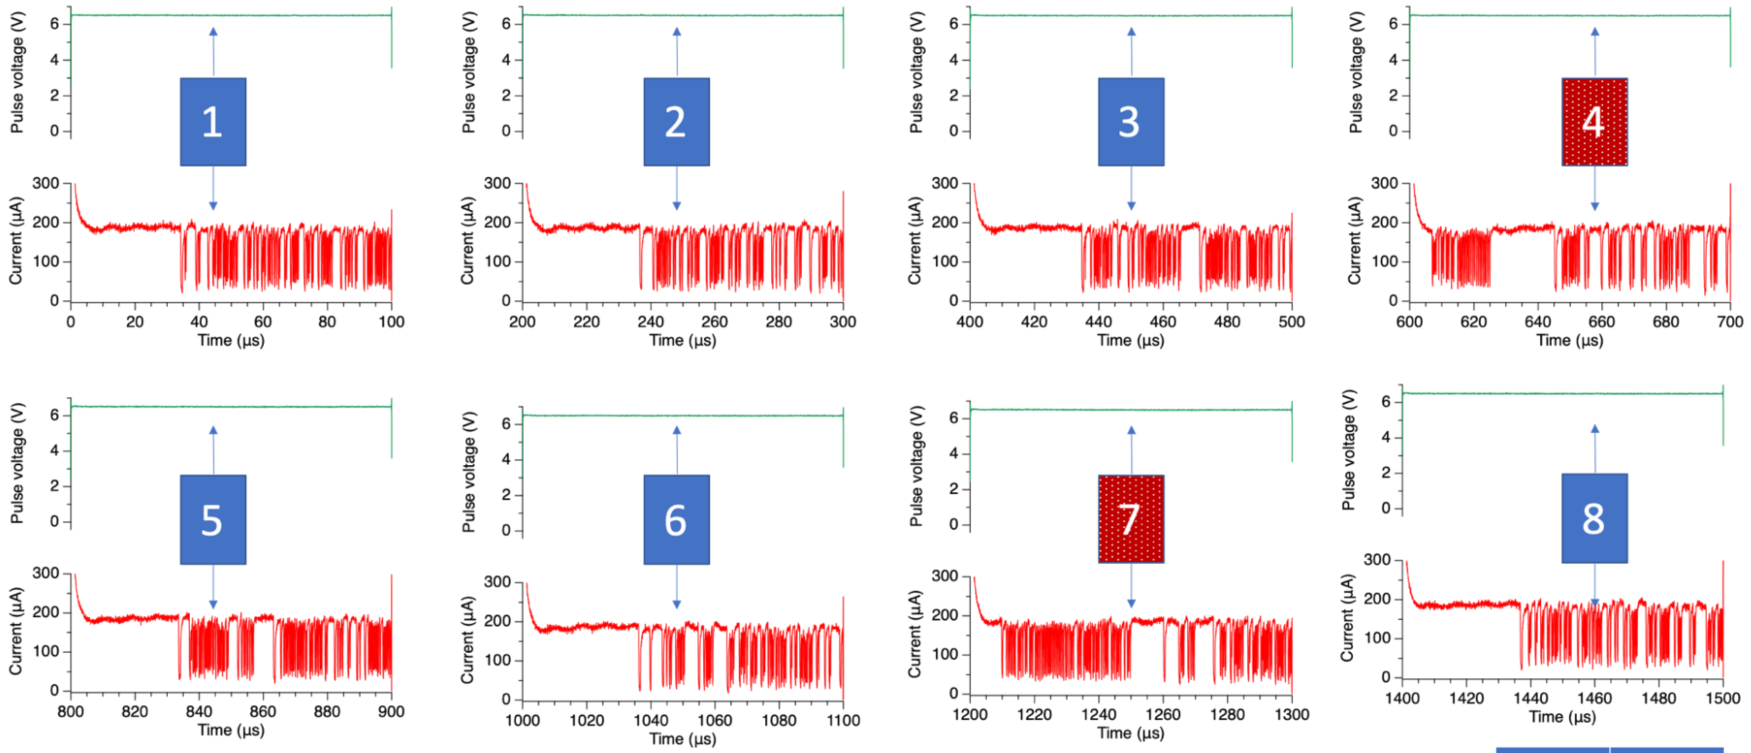


| Pulse | $t_{nuc}$ (μs) |
|---|---|
| 1 | 34.17 |
| 2 | 36.52 |
| 3 | 34.65 |
| 4 | 6.92 |
| 5 | 33.54 |
| 6 | 36.15 |
| 7 | 9.78 |
| 8 | 36.74 |

FIG. S6.2. Bubble-blockage signals for the 525-nm pore under a 6.45 V bias voltage and eight pulses. For two of these pulses (marked in red), early hetero nucleation is observed, while for all the other pulses, there is a long waiting time, after which a homo bubble nucleates.

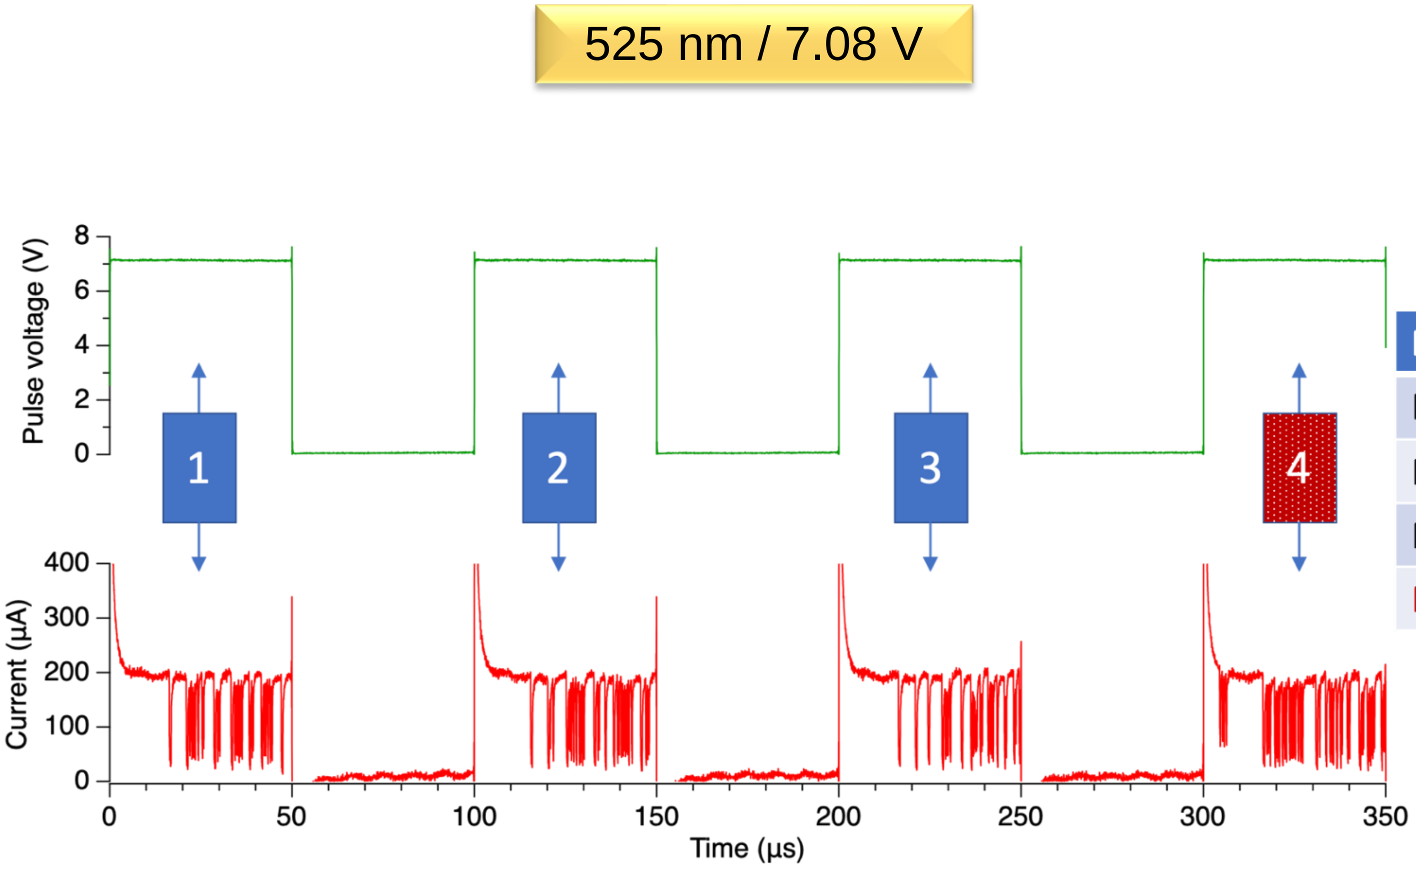


| Pulse | $t_{nuc}$ |
|---|---|
| Pulse 1 | 16.3 μs |
| Pulse 2 | 15.4 μs |
| Pulse 3 | 16.3 μs |
| Pulse 4 | 4.4 μs |

FIG. S6.3. Bubble-blockage signals for the 525-nm pore under a 7.08 V bias voltage and four pulses. Early hetero nucleation is observed for only one of these pulses, while for all the other pulses, there is a long waiting time, after which a homo bubble nucleates.

## 280 nm / 6.84 V

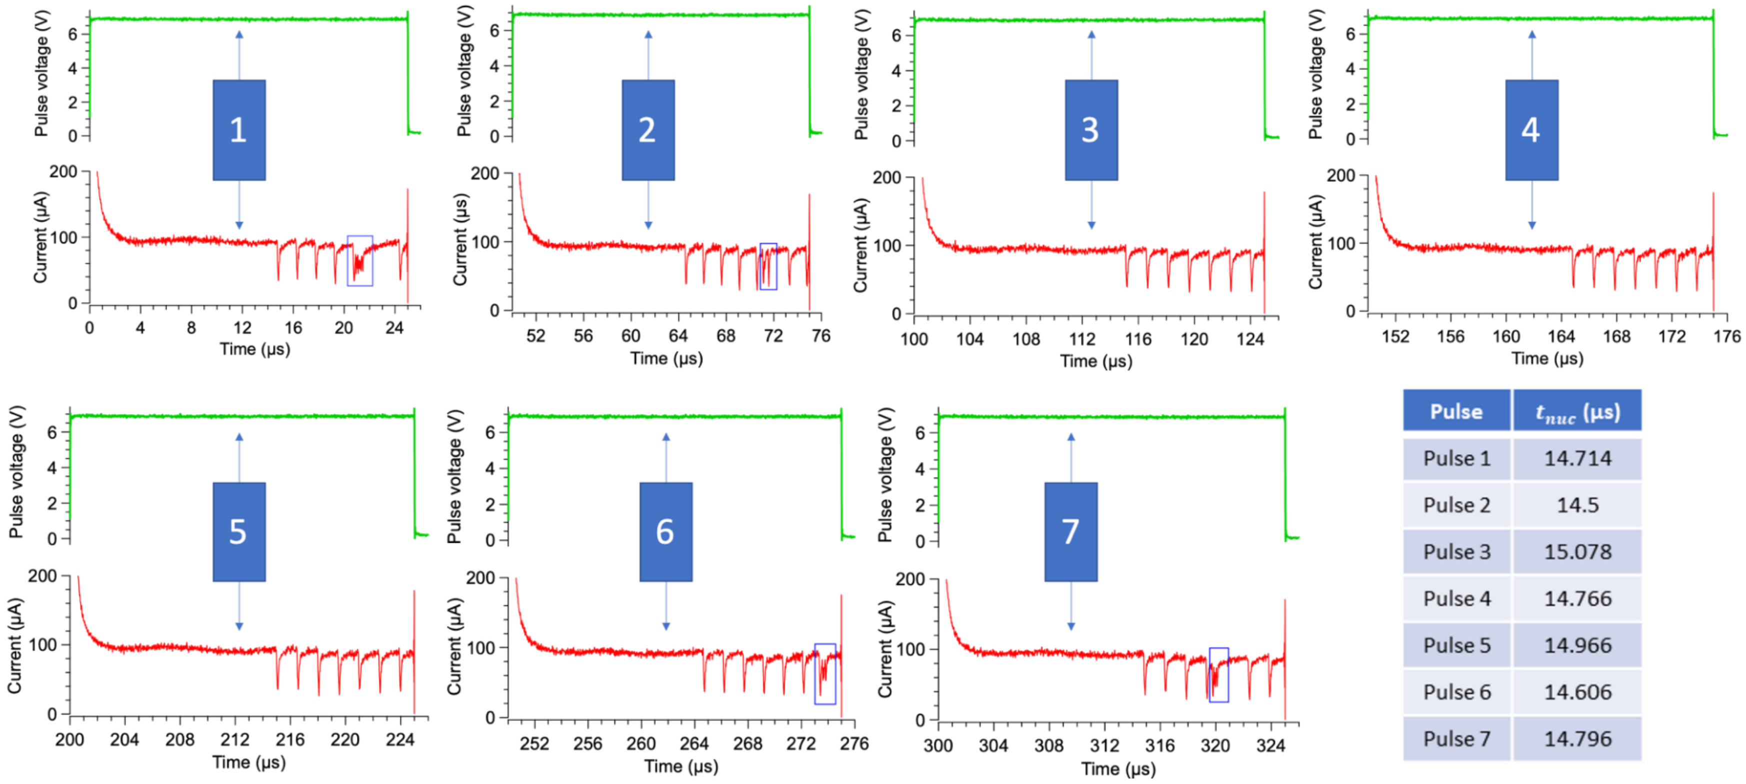


| Pulse | $t_{nuc}$ (μs) |
|---|---|
| Pulse 1 | 14.714 |
| Pulse 2 | 14.5 |
| Pulse 3 | 15.078 |
| Pulse 4 | 14.766 |
| Pulse 5 | 14.966 |
| Pulse 6 | 14.606 |
| Pulse 7 | 14.796 |

FIG. S6.4. Bubble-blockage signals for the 280-nm pore under a 6.84 V bias voltage and seven pulses. For all pulses, the bubbles start with a homo bubble after a similar waiting time. No early hetero nucleation is observed. However, for pulses 1, 2, 6, and 7 we can find non-periodic hetero bubbles appearing in the reheating sequence (marked by blue squares). The occurrence of hetero bubbles is markedly lower than in the 525-nm pores.

# 7. Periodic bubble generation for expanded 280-nm pore

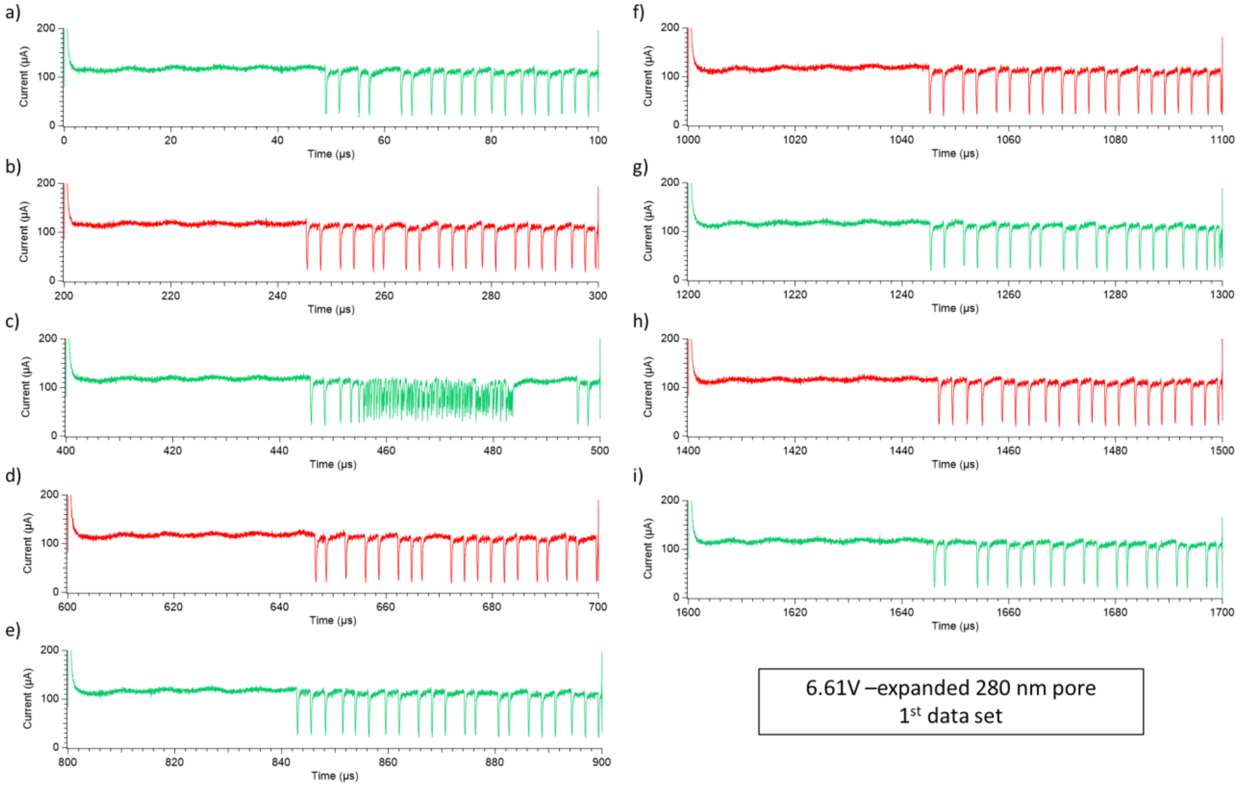


FIG. S7.1. Bubble generation sequence for an expanded 280-nm pore for 9 successive pulses during which bias voltages of 6.61 V were applied. These signals were captured after performing bubble generation experiments for approximately 1 hour on the initially 280-nm diameter pore. In most pulses, periodic homogeneous nucleation remained the dominant mode of bubble nucleation.

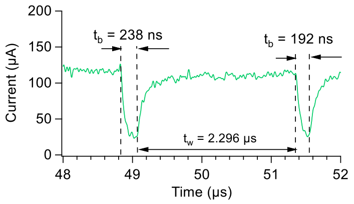

FIG. S7.2. Closeup of FIG. S7.1(a) for the first two bubbles. Due to pore expansion, the baseline current increased from 90 μA to 120 μA. The specific Joule heat, *H* reduces with expansion in pore diameter, thus the waiting period to reach the homogeneous nucleation temperature increased (2.30 µs for the expanded pore compared to 1.36 µs at initial state [FIG. 11a]). The increased waiting periods and pore diameter expansion led to extra sensible heat accumulation in the liquid. This caused bigger bubbles with larger blockage duration (~215 ns compared to ~120 ns in FIG. 11a).

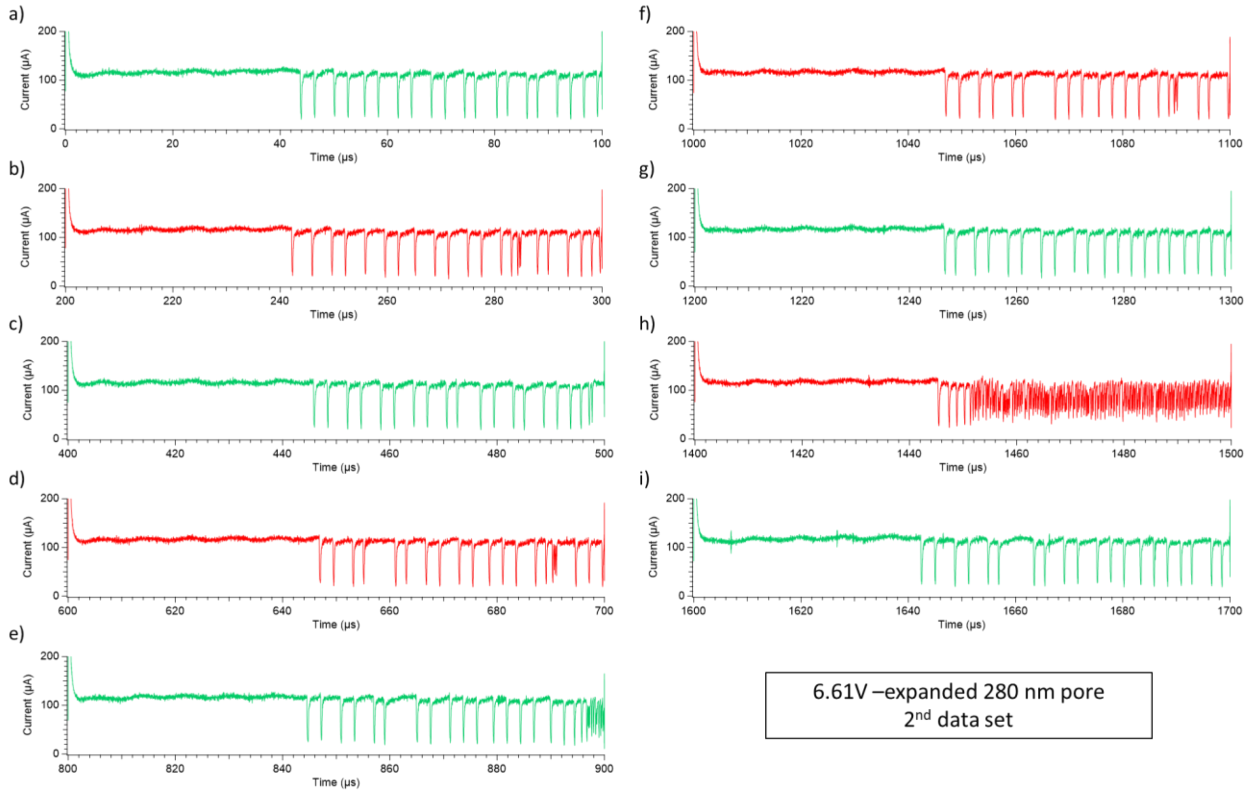


FIG.S7.3. Bubble generation sequence for an expanded 280-nm pore for 9 additional pulses during which bias voltages of 6.61 V were applied. In this case as well, most of the pulses showed periodic homogeneous bubble formation.

# 8. Nanopore reheating simulations

After a bubble-blockage event is complete, Joule heating is resumed, and the nanopore current rises as the temperature and ionic conductivity increase inside it. During this time, there is not a significant current contribution from capacitive charging, as the membrane was already fully charged during the initial heating. Moreover, as the blockage duration is more than an order of magnitude smaller than the initial heating time, the charge on the nanopore is not expected to significantly alter during the growth and collapse of the bubble. To simulate the transient current rise during reheating (resumption of Joule heating after a bubble event), we first obtained the temperature distribution of the liquid inside the nanopore post-bubble-collapse using one-dimensional (1D) bubble-dynamics simulations (Sec. 9). To obtain the temperature distribution in the silicon nitride membrane, we solved for thermal relaxation using Eq. (S8.1) from $t = t_{\mathrm{nuc}}$ to $t = t_{\mathrm{nuc}} + t_{\mathrm{lifetime}}$, where $t_{\mathrm{nuc}}$ and $t_{\mathrm{lifetime}}$ are the nucleation time in the experiments and the bubble lifetime obtained from bubble-dynamics simulations.

$$\rho_{\mathrm{SiN}x} c_{\mathrm{SiN}x} \frac{dT}{dt} = k_{\mathrm{SiN}x} \frac{1}{y} \frac{d}{dy}\left(y \frac{dT}{dy}\right) \tag{S8.1}$$

We employ an implicit 1D finite-difference scheme over 10 001 uniformly spaced grid points from $y = R_{\mathrm{p}}$ to $y = R_{\mathrm{p}} + 10$ µm with a 1-ns time spacing. The initial temperature distribution inside the membrane at $z = 0$ at $t = t_{\mathrm{nuc}}$ was obtained from the 2D axisymmetric Joule-heating simulations (Sec. 1). For the sake of simplicity, we assume no heat transfer between the liquid and the silicon nitride membrane during the blockage duration. So, in the bubble-dynamics simulation, we neglect the presence of the silicon nitride membrane altogether, and in the silicon nitride thermal relaxation, we apply the boundary conditions $\frac{dT}{dy} = 0$ at $y = R_{\mathrm{p}}$ and $T = T_0$ at $y = R_{\mathrm{p}} + 10$ µm. The solutions of the liquid temperature distribution from the bubble-

dynamics simulations and the membrane temperature from the thermal-relaxation model were used as the initial conditions for the reheating simulation. Figures S3.1(e) and S3.1(f) show the reheating current after the first bubble collapse for 7.08 V across the 525-nm-diameter pore and 6.84 V across the 280-nm-diameter pore, respectively. During this time, the simulated current matches the experimental trace to a better extent, demonstrating the validity of our models. It should be noted that the opening current post-collapse is almost two times that of the initial simulation current at the beginning of the pulse. This is because of the higher liquid temperature inside the nanopore, resulting in a higher electrical conductivity. Also, as the bubble grows and collapses, the sensible heat is spread over a wider area. Thus, the electrical conductivity in the access region of the pore is also high. This results in a low pore resistance, leading to high current flow through the nanopore and intense Joule heating, drastically reducing the waiting time before the subsequent bubble-nucleation event. For Fig. S3.1(e), after reheating of 4.18 μs, a second bubble nucleates homogeneously, at which point $T_c = T_{nuc}$ = 598 K, while for the 280-nm pore, $T_c$ reaches 570 K after 1.36 μs, when a second homogeneous bubble was observed [Fig. S3.1(f)].

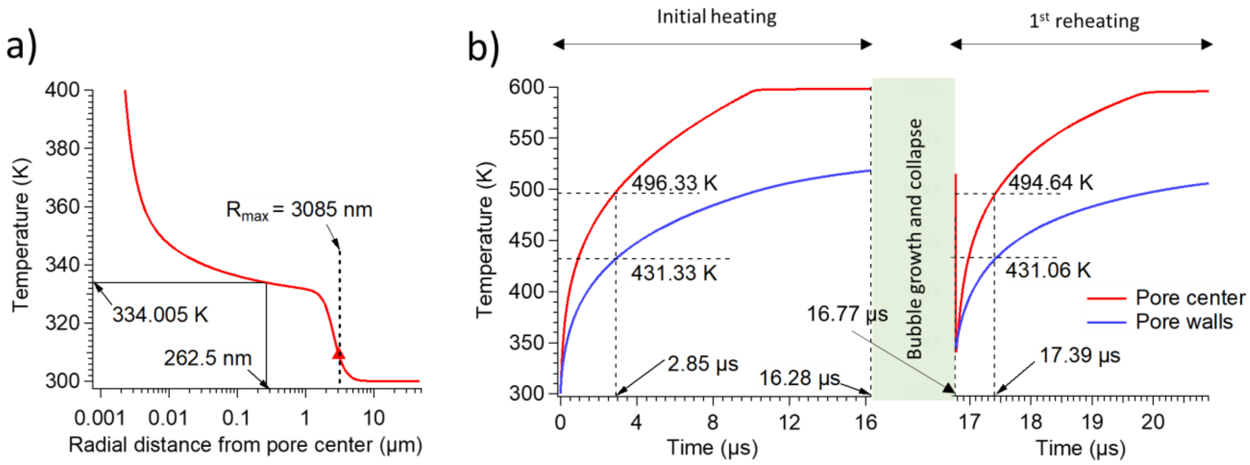


FIG. S8.1. (a) Radial temperature distribution after bubble collapse for the 525-nm pore under a 7.08-V bias. The asymptotic temperature distribution towards the pore center arises from rapid nanobubble collapse (luminescence), which dissipates rapidly during the

reheating time. (b) Transient development of temperature at the pore center and walls during the first heating cycle from 0 μs to 16.28 μs, followed by a bubble event of 490 ns. During this time, the bubble grows and collapses radially, while the bubble center remains stationary at the pore center. Furthermore, the thermal energy stored inside the silicon nitride membrane dissipates. After the bubble collapses, Joule heating recommences, and the average pore temperature rises from 335 K. According to our simulations, after 0.62 μs of reheating ($t$ = 17.39 μs), $T_w$ reaches 431.06 K and $T_c$ reaches 494.64 K [Fig. S8.1(b), right]. However, during the initial heating, it takes 2.85 μs for $T_w$ to reach 431.33 K [Fig. S8.1(b), left]. This longer heating time is because the pore was at ambient temperature before the pulse started. Due to the longer heating time, $T_c$ reaches the higher value of 496.33 K. Due to a shorter heating period during reheating, $\Delta T_p$ is shorter than that in the initial heating for the same value of $T_w$, making heterogeneous cluster nucleation more likely during the reheating time period.

# 9. Nanopore bubble dynamics

A 1D moving-boundary model, as proposed by Robinson *et al.* [11,12], was used to model homogeneous bubble growth. The bubble growth is assumed to be spherically symmetric. We simulate bubble growth starting from a critical nucleus at nucleation, which is given by

$$R_\mathrm{c} = \frac{2\gamma}{P_\mathrm{v} - P_\mathrm{w}}. \qquad \text{(S9.1)}$$

Here, the surface tension $\gamma$ and the saturation vapor pressure $P_\mathrm{v}$ are calculated at the nucleation temperature, $T_\mathrm{nuc}$. $P_\mathrm{w}$ is the atmospheric pressure. The nucleation temperature is equal to the liquid temperature at the pore center, $T_c$ (Fig. S4.1), at the experimentally obtained homogenous nucleation time, $t_\mathrm{nuc}$. A very small perturbation of the radius corresponding to the addition of one molecule to the critical nucleus disturbs the mechanical equilibrium and triggers bubble growth. The bubble growth is captured using the Rayleigh–Plesset equation,

$$R\frac{d^2R}{dt^2}+\frac{3}{2}\left(\frac{dR}{dt}\right)^2=\frac{1}{\rho}\left(P_\mathrm{v}-P_\mathrm{w}-2\frac{\gamma}{R}-4\frac{\mu_\mathrm{l}}{R}\frac{dR}{dt}\right). \quad \text{(S9.2)}$$

This equation has been derived in [13] by considering spherical bubble growth in an incompressible liquid with constant liquid density and viscosity and assumption of no mass transfer at interface. In our formulation, the temperature inside the bubble is assumed to be uniform, and this changes with time as the bubble grows under vapor influx. The vapor inside the bubble is assumed to be saturated, thus the vapor pressure $P_\mathrm{v}$ and the density $\rho_\mathrm{v}$ can be expressed as a functions of the saturated vapor temperature $T_\mathrm{v}$ (Fig. S9.1). The surface tension $\gamma$, dynamic viscosity of water $\mu_\mathrm{l}$, and liquid density $\rho$ are expressed as functions of the interface temperature (following the property–temperature relationships given in Figs. S9.1 and S2.2), which is equal to $T_\mathrm{v}$. During bubble growth, the vapor pressure is the driving force that causes the bubble to expand under the compressive forces of surface tension and ambient pressure. The mass balance of the bubble is captured by

$$\frac{d}{dt}\left(\rho_\mathrm{v}\frac{4\pi R^3}{3}\right)=\dot{m}4\pi R^2, \quad \text{(S9.3)}$$

where $\dot{m}$ is the vapor influx at the interface and $\rho_\mathrm{v}$ is the saturation vapor density. Eq. (S9.3) can be solved to obtain

$$\left(\rho_\mathrm{v}\frac{dR}{dt}+\frac{R}{3}\frac{d\rho_\mathrm{v}}{dt}\right)=\dot{m}. \quad \text{(S9.4)}$$

The mass flux at the interface originates from the evaporation of water under the temperature gradient across the thermal boundary layer,

$$\dot{m}=\frac{\kappa\left.\frac{dT}{dx}\right|_\mathrm{interface}}{h_\mathrm{fg}}, \quad \text{(S9.5)}$$

where $h_\mathrm{fg}$ is the latent heat of evaporation, modeled as a function of the saturation vapor temperature (Fig. S9.1).

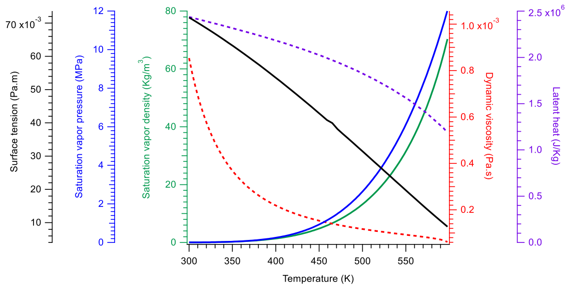


FIG. S9.1. Thermophysical properties evaluated as functions of temperature. Green: saturation vapor density [3]; blue: saturation vapor pressure [3]; black: surface tension [14]; red: dynamic viscosity [2]; and violet: latent heat capacity [14].

To calculate the temperature gradient at the interface, we solve the energy-conservation equation in the superheated liquid in a spherical co-ordinate system, which is given by

$$\frac{\partial T}{\partial t} + u\frac{\partial T}{\partial x} = \frac{1}{\rho c_\mathrm{p}}\left\{\frac{1}{x^2}\left[\frac{\partial}{\partial x}\left(x^2\kappa\frac{\partial T}{\partial x}\right)\right]\right\}, \tag{S9.6}$$

where $u$ is the radial velocity of the liquid and is calculated as

$$u = \frac{\rho|_R}{\rho|_x}\frac{R^2}{\mathrm{x}^2}\frac{dR}{dt}, \tag{S9.7}$$

where $x$ denotes the radial distance from the center of the nanopore and $\rho$ is a function of liquid temperature, which varies with position. Eq. (S9.6) is discretized using a second-order finite-difference scheme solved on a 1D mesh comprising of 151 computational nodes, as shown in Fig. S9.2. The computational nodes are distributed densely near the bubble surface, where the temperature gradient is high, and sparsely distributed far from the bubble surface, where the temperature gradient approaches zero. The location of the computational points is decided using the formula

$$R_{\mathrm{CN}}(i) = R + \frac{(R_\infty - R)(g^{i-1} - 1)}{g^N - 1}, \text{ for } 1 \le i \le 150 \qquad \text{(S9.8)}$$

$$R_{\mathrm{CN}}(i) = R_\infty, \text{ for } i = 151 \qquad \text{(S9.9)}$$

where $R_\infty$ = 50 µm, $g$ = 1.07, $N$ = 150, and $i$ is the index denoting the computational node. As the bubble grows, the computational grid gets compressed, as shown in Fig. S9.2(b). To solve Eq. (S9.6) using a traditional finite-difference scheme, we transformed the equation into a stationary grid with uniform grid spacing by using co-ordinate transformation metrics, as described by Robinson *et al.* [11].

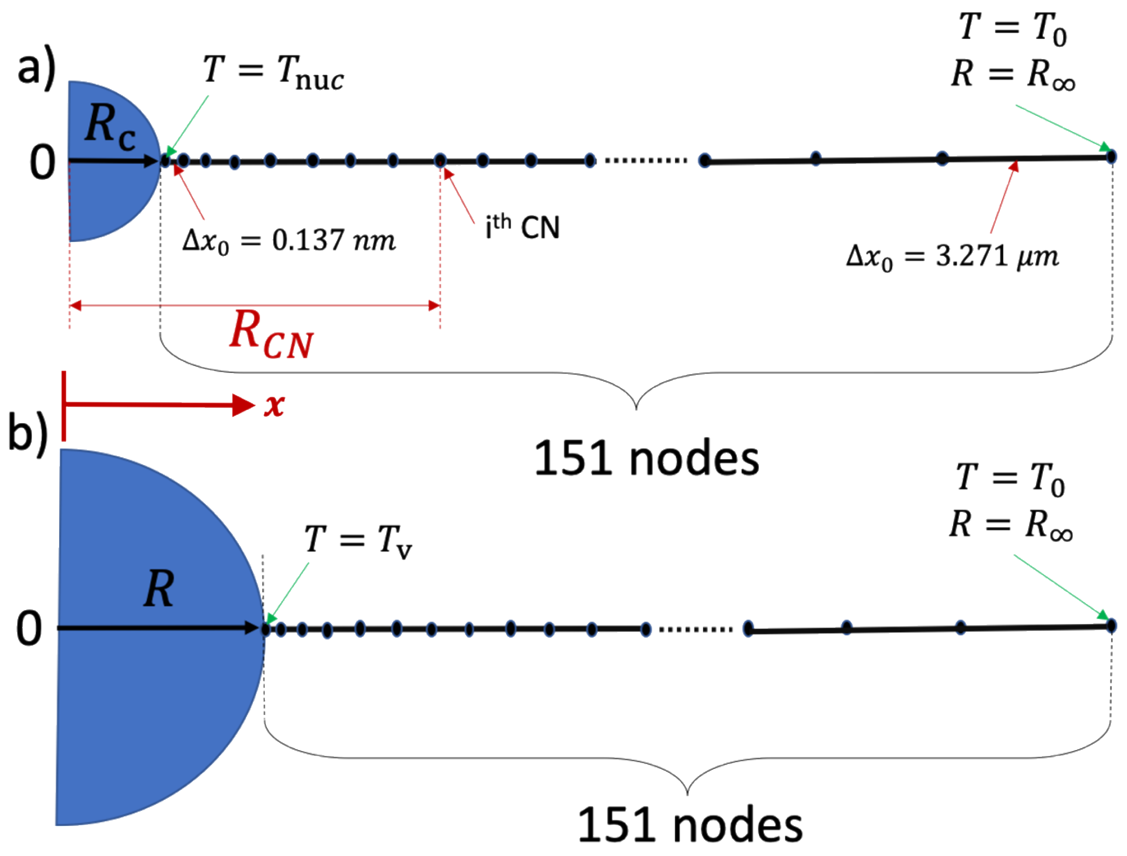


FIG. S9.2. Schematic of the 1D mesh on which Eq. (S9.6) is solved to obtain the liquid temperature distribution. (a) Mesh distribution at the nucleation point: 151 computational nodes are distributed radially, from the bubble surface to *x* = 46.73 µm from the bubble

surface. The mesh size varies from 0.137 nm at the bubble interface to 3.271 µm at the other end. (b) The mesh is compressed as the bubble grows.

The *z*-direction temperature distribution inside the nanopore at $t_{\mathrm{nuc}}$ obtained from the Joule heating-simulation (Fig. S9.3a) was interpolated over the 1D grid in the *x* direction (Fig. S9.2), which served as the initial conditions for bubble growth. At $t = t_{\mathrm{nuc}}$, a bubble of critical radius was inserted at the point of maximum temperature, which for a cylindrical nanopore is at its center (i.e., $x = 0$). The temperature distribution was shifted in the $+x$ direction using the formula

$$T_{t=t_{\mathrm{nuc}}}(x) = T_{t=t_{\mathrm{nuc}}}{}^{*}\left\{x - R_{\mathrm{c}}\left[1 - \left(\frac{\rho_{\mathrm{v}}(T_{\mathrm{nuc}})}{\rho(T_{\mathrm{nuc}})}\right)^{\frac{1}{3}}\right]\right\}. \quad \text{(S9.10)}$$

We assume that at nucleation, a sphere of liquid at the nucleation temperature evaporates and creates a spherical volume of vapor of equal mass. As the vapor sphere is bigger than the evaporating liquid sphere, the temperature distribution starting from the liquid sphere surface is translated by the offset amount to obtain the radial temperature distribution from the bubble surface. At superheating temperatures ~600 K, the ratio $\rho_{\mathrm{v}}/\rho = 0.2032$, and thus cannot be neglected. The parameter $T_{t=t_{\mathrm{nuc}}}$ is the temperature distribution after shifting, and $T_{t=t_{\mathrm{nuc}}}{}^{*}$ is the temperature distribution inside the nanopore along the pore axis ($+z$ direction) obtained as a result of Joule heating [Fig. S9.3(a)].

Transient bubble growth was solved in a loop in MATLAB. For each time step, first, Eq. (S9.6) was solved to update the temperature in the liquid. The temperature-dependent thermophysical properties were calculated at the temperatures from the previous time step. We used Dirichlet boundary conditions $T = T_{\mathrm{v}}$ at the bubble interface and $T = T_0$ at the other end of the 1D mesh, as shown in Fig. S9.2. From the updated temperature distribution, $dT/dx$ was calculated at the interface, which was used to obtain the vapor influx $\dot{m}$ using Eq. (S9.5). Eqs. (S9.2) and (S9.4) were simultaneously solved using a fourth-order Runge–Kutta method

to obtain the bubble radius $R$, growth rate $\dot{R}$, and vapor temperature $T_v$. Using the updated value of $R$, the 1D grid was re-meshed using Eqs. (S9.8) and (S9.9), and the grid transformation metrics for Eq. (S9.6) [11, 12] were re-calculated. Next, Eq. (S9.6) was solved to obtain the temperature distribution in the liquid for the next time step using the updated vapor temperature as the boundary condition at the bubble interface. In this way, the simulation progressed. The time spacing was chosen for each time step such that: i) the interface growth or shrinkage was less than or equal to 20% of the grid spacing at the interface, and ii) the vapor evaporated or condensed at the interface accounted for less than or equal to 20% of the grid spacing at the interface. Mathematically,

$$\Delta t_n = \min\left\{10^{-(3\exp(-0.003n)+11)}, 0.2\frac{\Delta x_{\text{interface}}}{|dR/dt|_{n-1}}, 0.2\frac{\rho\Delta x_{\text{interface}}}{|\dot{m}|_{n-1}}\right\}, \qquad \text{(S9.11)}$$

where $n$ denotes the time-step index.

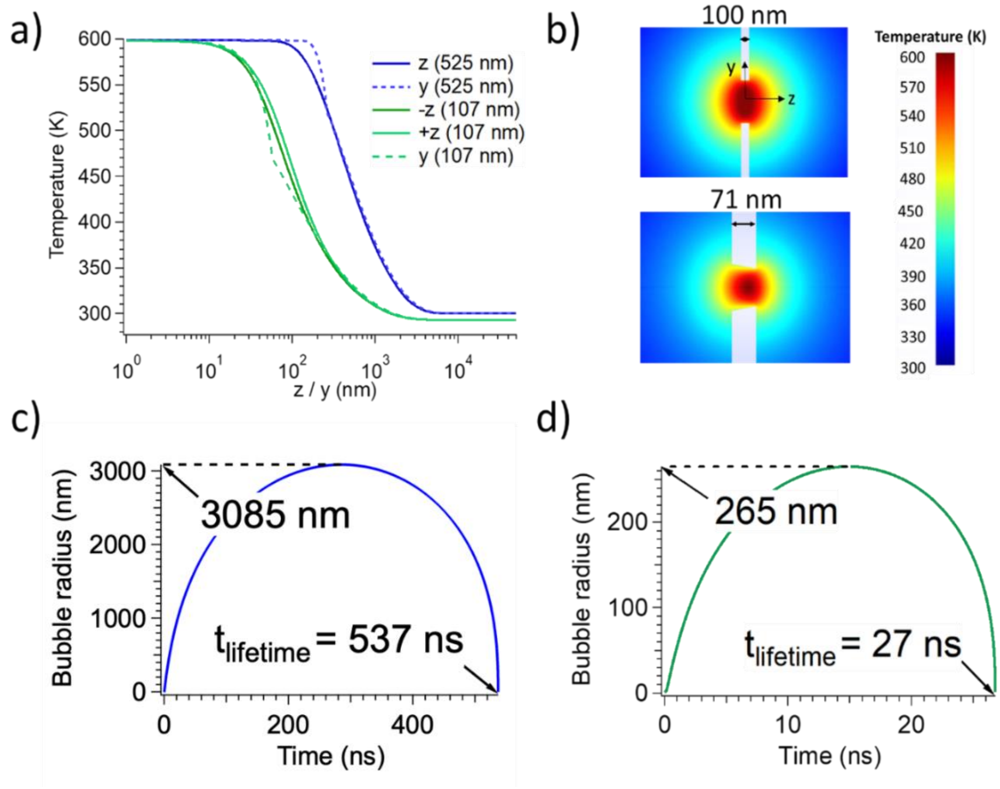

FIG. S9.3. (a) Temperature distribution inside the 525-nm pore at $t_{nuc}$ = 16.3 µs under a bias voltage of 7.08 V (blue) and inside the 107-nm pore [1] at $t_{nuc}$ = 10.4 µs under a bias voltage of 8.22 V (green). (b) Temperature distribution at $t_{nuc}$ for the 107-nm pore (top) and for the 525-nm pore (bottom). Bubble growth and collapse is simulated by considering the *z*-direction temperature distribution for (c) the 525-nm pore and (d) the 107-nm pore. According to our model, a bubble lifetime of 27 ns was estimated for the 107-nm pore compared to the 16 ns blockage duration observed by the previous study of Levine *et al.* [1].

# References


[1] E. V Levine, M. M. Burns, and J. A. Golovchenko, Phys. Rev. E **93**, 13124 (2016).

[2] IAPWS, *Release on the IAPWS Formulation 2008 for the Viscosity of Ordinary Water Substance* (2008).

[3] W. Wagner and A. Pruß, J. Phys. Chem. Ref. Data **31**, 387 (2002).

[4] A. Rogacs and J. G. Santiago, Anal. Chem. **85**, 5103 (2013).

[5] S. P. Porras, M. L. Riekkola, and E. Kenndler, Electrophoresis **24**, 1485 (2003).

[6] E. R. Nightingale, J. Phys. Chem. **63**, 1381 (1959).

[7] J. E. Bannard, J. Appl. Electrochem. **5**, 43 (1975).

[8] D. J. E. Harvie, ANZIAM J. **52**, 1126 (2012).

[9] V. Dimitrov, U. Mirsaidov, D. Wang, T. Sorsch, W. Mansfield, J. Miner, F. Klemens, R. Cirelli, S. Yemenicioglu, and G. Timp, Nanotechnology **21**, 065502 (2010).

[10] M. Soleimani, R. J. Hill, and T. G. M. Van De Ven, Langmuir **29**, 14168 (2013).

[11] A. J. Robinson and R. L. Judd, Int. J. Heat Mass Transf. **47**, 5101 (2004).

[12] A. J. Robinson and R. L. Judd, Int. J. Heat Mass Transf. **44**, 2699 (2001).

[13] C. E. Brennen, *Cavitation and Bubble Dynamics* (2013).

[14] W. M. Haynes, *CRC Handbook of Chemistry and Physics* (2016).
